# Supplementary material for: Renormalization Group Summation at High Orders and Implications to the Determination of Some Standard Model Parameters
Source: arXiv:2311.06577 source file (2023-11-11)
Supplement: Supplementary file 1 [file AppendixB.tex]

\chapter{Appendix 2} % Main appendix title

\label{Appendix B} % Change X to a consecutive letter; for referencing this appendix elsewhere, use \ref{AppendixX}

\lhead{Appendix B. \emph{tables}} % Change X to a consecutive letter; this is for the header on each page - perhaps a shortened title
